# Supplementary material for: Learning and Sampling of Atomic Interventions from Observations
Source: arXiv:2002.04232 source file (2020-08-05)
Supplement: Supplementary file 1 [file appendix.tex]

\newpage
\appendix

\section{Learning algorithm for Bayesian Networks}\label{sec:app-bn}

In this section we present Algorithm~\ref{algo:bn} for an unknown small indegree $\le d$ bayes nets $P$ over the sample space $\{0,1\}^n$ on a known graph $G$ on vertex set $[n]$. The Laplace corrected empirical estimator takes $z$ samples from a distribution over $k$ items and assigns to item $i$ the probability $(z_i+1)/(z+k)$ where $z_i$ is the number of occurrences of item $i$ in the samples. We in fact give learning algorithm in KL distance, defined as $KL(P,Q)=\sum_i P(i) \ln {P(i) \over Q(i)}$. From Pinsker's inequality $\dtv^2(P,Q) \le 2 KL(P,Q)$, a $\dtv$ learning result follows.

%\begin{figure}
\begin{algorithm}
\SetKwInOut{Input}{Input}
\SetKwInOut{Output}{Output}
\Input{Samples from an unknown bayes net over $\{0,1\}^n$ on a known graph $G$ of indegree $\le d$, parameters $m,t$}
\Output{A bayes net $Q$ over $G$}
Take $m$ samples from the bayes net\;
\For{every vertex $i$}{
\For{every fixing of its parents $a$}{
$N_{i,a} \gets$ the number of samples where $i$'s parents are $a$\;
\eIf{$N_{i,a} \ge t$}{
$Q(i\mid a) \gets$ the empirical distribution of the samples where $i$'s parents are $a$ with laplace correction\;
}{
$Q(i\mid a) \gets$ uniform bit\;
} 
}
}
\caption{Bayes net learning}
\label{algo:bn}
\end{algorithm}
%\end{figure}

\subsection{Constant Success Probability}
\begin{theorem}\label{thm:bnlearningapp}
For $m= 24n2^d \log (n2^d)/\epsilon$ and $t=12\log (n2^d)$, \cref{algo:bn} satisfy $KL(P,Q)\le 5\epsilon$ with probability at least 2/3 over the randomness of sampling.
\end{theorem}
\begin{proof}
We set $m=24n2^d \log (n2^d)/\epsilon$ and $t=12\log (n2^d)$.
For every vertex $i$, for every fixing $a$ of its parents, let $\Pi[i,a]$ denote the event that parents of $i$ takes value $a$. We call a tuple $(i,a)$ {\em heavy} if $P[\Pi[i,a]]\ge \epsilon/n\cdot 2^d$ and {\em light} otherwise. Let $N_{i,a}$ denote the number of samples where $i$'s parents are $a$. We use the following subadditive result from~\cite{DBLP:conf/colt/CanonneDKS17}.
\begin{theorem}
$$KL(P,Q) \le \sum_{i} \sum_a P[\Pi[i,a]] KL(P(i\mid a),Q(i\mid a))$$
\end{theorem}
We also use the following result for learning a distribution in $KL$ distance.
\begin{theorem}[\cite{pmlr-v40-Kamath15}]\label{thm:exKLlearn}
Let $D$ be an unknown distribution over $k$ items.  Let $\hat{D}$ be the Laplace corrected empirical distribution of $z$ samples from $D$. Then $\ex{KL(D,\hat{D})} \le (k-1)/(z+1)$.
\end{theorem}

Henceforth we condition on the event that  ``all $(i,a)$ tuples which satisfy $N_{i,a}\ge t$ also satisfy $N_{i,a}\ge n2^dP[\Pi[i,a]]t/\epsilon$". From Chernoff's and union bound with our choice of $m$ and $t$ all heavy tuples satisfy both the statements except 1/20 probability. By definition of light items any light item with $N_{i,a}\ge t$ also satisfy this.

Items which do not satisfy $N_{i,a}\ge t$ must be light for which $KL(P(i\mid a),Q(i \mid a)) \le p\ln 2p + (1-p)\ln 2(1-p) \le 1$ where $p=P[i=1|a]$, since in that case $Q(i \mid a)$ is the uniform bit. 

\cref{thm:exKLlearn} gives us $\ex{KL(P(i\mid a),Q(i\mid a))} \le \epsilon/12n2^dP[\Pi[i,a]]$ for items with $N_{i,a}\ge t$.
We get $\ex{KL(P,Q)}\le \sum_{(i,a) \text{ heavy}} \epsilon/12n2^d + \sum_{(i,a) \text{ light}} \epsilon/n2^d \le 1.1\epsilon$. The theorem follows from Markov's inequality.

\end{proof}

\begin{corollary}
There is an algorithm which given $m\ge 24n|\Sigma|^{d+1} \log (n|\Sigma|^{d+1})/\epsilon$, samples from a bayes net $P$ over $\Sigma^n$ on a graph $G$ of indegree at most $d$ return a bayes net $Q$ on $G$ such that $KL(P,Q) \le \epsilon$ with probability 2/3.
\end{corollary}
\begin{proof}
We can encode each $\sigma\in \Sigma$ of the bayes net as a $\log |\Sigma|$ size boolean string which gives us a bayes net of degree $(d+1) \log |\Sigma|$ over $n\log |\Sigma|$ variables. Then we apply Theorem~\ref{thm:bnlearningapp}
\end{proof}

\subsection{Very High Success Probability}
\begin{theorem}\label{thm:bnlearningapphigh}
For $m= \Theta(n2^d\log ({n2^d\over \delta})/\epsilon)$ and $t=\Theta(\log ({n2^d\over \delta}))$ with appropriate choice of constants \cref{algo:bn} satisfy $KL(P,Q)=O(\epsilon)$ with probability at least $1-2\delta$ over the randomness of sampling.
\end{theorem}
\begin{proof}
We set $m= \Theta(n2^d\log ({n2^d\over \delta})/\epsilon)$ and $t=\Theta(\log ({n2^d\over \delta}))$, choosing the constant appropriately so that the rest of the proof goes through.
For every vertex $i$, for every fixing $a$ of its parents, let $\Pi[i,a]$ denote the event that parents of $i$ takes value $a$. We call a tuple $(i,a)$ {\em heavy} if $P[\Pi[i,a]]\ge \epsilon/n\cdot 2^d$ and {\em light} otherwise. Let $N_{i,a}$ denote the number of samples where $i$'s parents are $a$. We use the following subadditive result from~\cite{DBLP:conf/colt/CanonneDKS17}.
\begin{theorem}
$$KL(P,Q) \le \sum_{i} \sum_a P[\Pi[i,a]] KL(P(i\mid a),Q(i\mid a))$$
\end{theorem}
We also use the following result for learning a distribution in $KL$ distance.
\begin{theorem}[\cite{canonne-writeup}]\label{thm:highKLlearn}
There is an algorithm that takes $O((k+\log {1\over \delta})/\epsilon)$ samples from an unknown distribution $D$ over $k$ items and returns a distribution $\hat{D}$ such that $KL(D,\hat{D})\le \epsilon$ with probability at least $1-\delta$.
\end{theorem}

Henceforth we condition on the event that  ``all $(i,a)$ tuples which satisfy $N_{i,a}\ge t$ also satisfy $N_{i,a}\ge n2^dP[\Pi[i,a]]t/\epsilon$". From Chernoff's and union bound with our choice of $m$ and $t$ all heavy tuples satisfy both the statements except $\delta$ probability. By definition of light items and $t$, any light item with $N_{i,a}\ge t$ also satisfy this.

Items which do not satisfy $N_{i,a}\ge t$ must be light for which $KL(P(i\mid a),Q(i \mid a)) \le p\ln 2p + (1-p)\ln 2(1-p) \le 1$ where $p=P[i=1|a]$, since in that case $Q(i \mid a)$ is the uniform bit. 

\cref{thm:highKLlearn} gives us $KL(P(i\mid a),Q(i\mid a)) \le O(\epsilon/n2^dP[\Pi[i,a]])$ for items with $N_{i,a}\ge t$ except $\delta$ probability.
We get $KL(P,Q)\le \sum_{(i,a) \text{ heavy}} O(\epsilon/n2^d) + \sum_{(i,a) \text{ light}} \epsilon/n2^d = O(\epsilon)$ except $2\delta$ probability in total.

\end{proof}

\begin{corollary}
There is an algorithm which given $m= O(n2^dP[\Pi[i,a]]\log ({n2^d\over \delta})/\epsilon)$, samples from a bayes net $P$ over $\Sigma^n$ on a graph $G$ of indegree at most $d$ return a bayes net $Q$ on $G$ such that $KL(P,Q) \le \epsilon$ with probability $1-\delta$.
\end{corollary}
\begin{proof}
We can encode each $\sigma\in \Sigma$ of the bayes net as a $\log |\Sigma|$ size boolean string which gives us a bayes net of degree $(d+1) \log |\Sigma|$ over $n\log |\Sigma|$ variables. Then we apply Theorem~\ref{thm:bnlearningapphigh}
\end{proof}
